# Supplementary material for: The Currents of Conflict: Decomposing Conflict Trends with Gaussian Processes
Source: arXiv:2506.06828 source file (2025-06-07)
Supplement: Supplementary file 1 [file appendices.tex]

\section{Online appendix}\label{online_app}

\subsection{Data -- online appendix}

% Using Views rep data 
To estimate the patterns of conflict I need data which is highly disaggregated at both the temporal and spatial level. I also want data used by similar forecasting efforts in order to ensure a valid basis of comparison. Using the replication data available from \cite{hegre2019views} fulfills these demands while also facilitating a suitable point of reference.\par

% PRIO
\cite{hegre2019views} use the PRIO-grid as basis for the spatial dimension \citep{prio_code_2015}. It is a global grid constituted by $0.5\times0.5$ decimal degree cells -- squares roughly measuring $50km\times50km$ at the equator \citep[367]{Tollefsen_2012}. \cite{hegre2019views} use a geographical subset of the full PRIO-grid -- specifically the grid covering Africa. For comparability I use the same geographical subset.\par

% UCDP
To obtain data on conflict events, \cite{hegre2019views} use the UCDP which contains dates, coordinates and fatality-counts pertaining to violent conflicts. Specifically \cite{hegre2019views} use the feature \emph{best} which denotes \enquote*{The best (most likely) estimate of total fatalities resulting from an event} \cite[7]{Croicu_Sundberg_2017}. \cite{hegre2019views} focuses on \emph{state-based conflict} (sb), i.e \enquote*{a contested incompatibility that concerns government and/or territory where the use of armed force between two parties, of which at least one is the government of a state, results in at least 25 battle-related deaths in a calendar year.} \citep{Croicu_Sundberg_2017}. \cite{hegre2019views} aggregate these fatalities at a monthly level. For comparability I here use the same temporal unit of analysis and focus on the same subset of conflicts.\par

% The y/X
As such, all data used from in this effort comes from this single measure $best_{sb}$. All features are derived from this measure and all targets are based on it: Past patterns will be used to predict future patterns. I take the logarithm of $best_{sb}$ to create a measure of \emph{conflict magnitude} ($cm$). On a theoretical level The log-transformation is warranted in order to lessen the impact of extreme outliers and because it appears theoretically prudent: We would expect a change from $0$ to $100$ fatalities to prove more disruptive than a change from $1,000$ to $1,100$ fatalities. On a more practical level out-of-sample validation showed much better performance when applying this transformation. The measure $cm$ will first be used to estimate and extrapolate temporal and spatial patterns conflict. These estimated and extrapolated patterns will then be used as features in a final machine learning algorithm. To create the target for this final step I follow \cite{hegre2019views} and apply a binary transformation of the original measure $best_{sb} > 0 := 1$, denoting whether or not some unit-of-analysis experience conflict or not.\par

% train/val/test
In order to evaluate the performance of my approach I use \emph{out-of-sample} prediction \citep{Ward_Greenhill_Bakke_2010, Goldstone_2010, hegre2019views}. Again I model my approach directly after \cite{hegre2019views}. Version $18.1$ of the UCDP dataset covers the years $1989 - 2017$. \cite{hegre2019views} use data from $1990$ through $2011$ for training while data from $2012$ through $2014$ is used for calibration and out-of-sample validation. During the final evaluation, the training and validation set are combined into a larger training set ($1990$ through $2014$) and the last $36$ months of data ($2015$ through $2017$) are used as a \emph{hold-out test set} for out-of-sample evaluation \citep[163]{hegre2019views}. For comparability, I use the exact same time-frame and train/validation/test splits as employed by \cite{hegre2019views}. My approach, however, can easily handle topical data directly obtained from PRIO and UCDP if need be.\par

\subsection{Feature selection -- online appendix}

% forward feature selection
To avoid an exhaustive search I use \emph{forward feature selection} to find the subset of features with the highest predictive power. This brings the number of feature combinations needed to be evaluated down from $65.535$ ($2^{16}-1$) to $136$ ($\frac{16\times(16+1)}{2}$) \citep[138-139]{herlau2016introduction}. First, I use a Random Forest model to choose the single best feature for prediction using the validation set. Having chosen that feature I now go on to find the second feature that improves the model the most (or impairs the model least). I iterate these steps until all features are exhausted. I then asses when the marginal benefit of adding more features evaporates. The convention is to stop when the results worsen the first time \citep[138-139]{herlau2016introduction}. In this case the first dip in performance happens at five features making the first four features the selected subset.\par

\subsection{The Random Forest ensemble -- online appendix}

% what?
Having selected four specific features to represent the patterns of conflict, I need a supervised machine learning algorithm which can combine these patterns into a final forecasts. I follow \cite{hegre2019views} and construct a ensemble of $1,000$ Random Forest models. Random Forest models are themselves ensembles but tying them together in an even larger ensemble has some advantage not least pertaining to evaluation. Firstly, it discourages overfitting \citep{Gelman_2013, Mcelreath_2018} which is one of the reasons this is also done in \cite[163-164]{hegre2019views}. As such, this choice facilitates better comparison. Secondly, having an ensemble of models provides me with a sample of predictions to evaluate. Naturally I can use the mean of the individual cell predictions as point estimates for my forecasts, but I can also evaluate the complete distributions of predictions across the samples. This reveals how sensitive the results are to the stochasticity of the Random Forest models.\par

% The range of hyper-parameters you iterate over
Furthermore, I let the hyper-parameters of the individual Random Forest model vary slightly between each model. The specific ranges of hyper-parameters was selected via a random search doing the validation step. Instead of only using the single set of best-performing hyper-parameters, I chose a range for each hyper parameter that appeared to do reasonably well while still leading to some variance in predictions across models. This reveals how sensitive the results are to the specifications of the Random Forest models.\par

% differences to ViEWS:
The ensemble differs from \cite{hegre2019views} in two minor aspects. Firstly I do not use any undersampling as it -- somewhat surprisingly -- led to noticeable loss of predictive power. \cite{hegre2019views} incorporate undersampling to improve their predictive power and thus the omission of the step does not impede comparison. Secondly, I do not calibrate the predicted probabilities. Calibration is important for operational settings, but it does not change the conclusions when we are comparing predictive power. As such, this element is omitted to keep my effort concise.\par

\subsection{Principle metrics -- online appendix}
The primary evaluation metric used is the \emph{precision-recall} ($PR$) curve and the three related metrics \emph{recall}, \emph{precision} and the \emph{average precision} ($AP$) score. I will also use the \emph{Receiver Operating Characteristic} ($ROC$) curve along with the corresponding metric, the \emph{Area Under the Curve} ($AUC$) score \citep{Friedman_2001, He_2008}. Using multiple metrics to evaluate model performance is warranted, since model performance is inherently multi-dimensional \citep[165]{hegre2019views}.\par

% Introducing $AUC$ (and TO/TN/FN/FP)

% ROC and AUC
The $ROC$-curve and the $AUC$-score have been widely used in conflict studies \citep[14]{chadefaux2017conflict}. The $ROC$-curve does not require any hard thresholds to be set, which is advantageous since estimated probabilities are far more informative than binary classifications. It denotes the trade-off between the \emph{true positive rate} ($TP_{rate}$) and the \emph{false positive rate} ($FP_{rate}$) by plotting the $TP_{rate}$ over the $FP_{rate}$. This curve can be summarised by the area under it (the $AUC$-score) \citep[1277-1278]{He_2008}. The $ROC$-curve and $AUC$-score, however, tend to judge model-performance on highly imbalanced data overly favourable \citep[1278]{He_2008}. These metrics also favour models apt at classifying non-events if these constitutes the majority class \citep[165]{hegre2019views} -- which is not here our priority. As such, it cannot stand alone.\par  

% Introducing Precision, Recall, $PR$-curve and average precision.
The $PR$-curve shares many similarities with the $ROC$-curve but addressees its shortcomings. It gives a more honest evaluation of model performance on imbalanced data \citep[1278]{He_2008} and always prioritises events \citep{He_2008, su2015relationship} which is what we are interested in when forecasting conflicts \citep[165]{hegre2019views}. The $PR$-curve also denotes the trade off between two measures: $recall$ and $precision$. $Recall$ is just another name for the $TP_{rate}$ rate, while $precision$ denotes the rate of True Positives out of all Positives. Denoting True Positives $TP$, False Positives $FP$ and False Negative $FN$, $recall$ ($R$) and $precision$ ($P$) can be expressed according to equation \ref{eq:recall/precision}.\par

\[
P = \frac{TP}{TP+FP}; \quad R = \frac{TP}{TP+FN} \tag{13} \label{eq:recall/precision}
\]

% Average precision
The $PR$-curve can also be summarised by the area under the curve ($AUPR$) or an equivalent unbiased estimation of this area called average precision $AP$ \citep{boyd2013area, su2015relationship}. The key difference between $AUC$ and $AP$ is that the latter places more emphasis on identifying high probability events than identifying low probability events \citep[350]{su2015relationship} -- i.e. actual conflict events. This is also the reason \cite{hegre2019views} prioritizes this measure over $AUC$. Another notable difference is that an $AUC$-score of $0.5$ denotes a classifier which is no better than random, where an $AP$-score of $0.5$ can be decent depending on the context \citep[350-351]{su2015relationship}. An approximation of the \enquote*{random} baseline of $AP$ is given the share of events \citep[132]{bestgen2015AP}. If the data is precisely balanced, the random baseline for the $AP$-score is $0.5$ just like the $AUC$-score. If the data is imbalanced, say $5\%$ events, the random baseline for the $AP$-score will be $0.05$. The $AP$-score can be expressed as seen in equation \ref{eq:ap} where $R_n$ and $P_n$ are the precision and recall at the $n^{th}$ threshold \citep{scikit-learn}.\par

\[
AP = \sum_n (R_n-R_{n-1})P \tag{14} \label{eq:ap}
\]

% The downside and the solution
The downside of $AP$ is that it is not particularly interpretable on a substantive level \citep[251]{hegre2017evaluating}. As such, to best present the potential of my framework in substantial terms, the $AP$-score will be used together with $recall$ and $precision$. Furthermore, the components $TP$, $FP$, $FN$ and $TN$ will be used for visualisations.\par

\subsection{Future perspectives -- online appendix} % maybe put in online appendix

% what
Within the larger field of Peace Research, Conflict forecasting is an important and growing field in rapid development. The approach here presented contribute to this field by showing how we might estimate tempo-spatial conflict exposure and simultaneously harness unprecedented levels of predictive power from past conflict patterns. Notably, the high performance of the presented approach also generate a number of future perspectives.\par

% Into ViEWS
The apparent next step is to incorporate the competent here produced into larger frameworks such as ViEWS. This will naturally allow us to survey the extent to which my approach generates novel information versus capturing information already contained in other, more structural, components. This will also allow us to update our assessment regarding the importance of conflict exposure for the continuation, diffusion, and reemerging of conflicts.\par

% the travel problem.
Secondly, given the predictive power of past patterns, future studies should survey whether these patterns generalize. Following \citet{hegre2019views} I here focused on Africa yet it is uncertain whether the specifications identified, the hyper-parameters estimated and the features selected will perform comparatively well given other regions. Indeed, it is very possible that Africa is already too large a geographic region for my approach to achieve its full potential. It is likely that temporal and spatial patterns differ between different regions due to geography and social/economic factors. For instance some regions might exhibit clear seasonal trends while others does not. Thus, future studies might asses the potential of using more geographically local models and/or hierarchical model structures.\par

% different forecast windows
Thirdly, using distinct models for different forecasting windows will likely also improve forecasting. One of the benefits of the approach here presented is that we know how far into the future our features provides relevant information. As such, various short term features might be more useful given a shorter forecasting window and ignored when using longer forecasting windows. In essence, if we have short and long term trends we should have short and long term forecasts well.\par  

% Regression
Lastly, while I here exemplify the potential of my approach on a classification task, the approach is also well suited for regression tasks. That is forecasting the magnitude of conflicts instead of, or along with, the probability of conflict. Indeed, I would argue that conflict forecasting is inherently a regression task and not a classification task. When using data from sources such as the UCDP we do have an countable target: Conflict fatalities ($y \in \mathbb{W}$, potentially logged). The \enquote*{binaryfication} creating a feature denoting conflict/non-conflict is artificial. We apply this transformation because we want to estimate the probability of conflict, but forecasting the magnitude of future conflicts appears just as paramount. Perhaps even more so when generating highly disaggregated forecast, as policy makers and actors now have the opportunity to formulate very specific strategies.\par
